# Supplementary material for: A Probabilistic Simulator of Spatial Demand for Product Allocation
Source: arXiv:2001.03210 source file (2020-01-09)
Supplement: Supplementary file 1 [file appendix.tex]

\appendix
\section{Appendix}

\subsection{Hyperparameters}
We detail the hyperparameter settings used in our implementations of \texttt{PSD-sim} and DQN.

\subsubsection{PSD-sim Priors}

\begin{itemize}

        \item $\boldsymbol{\mu_r}= [0, .. 0]^{\top}$
        \item $\gamma = 25$

        \item $\boldsymbol{\delta}_p= [2.5 , .. 2.5 ]^{\top}$
        \item $\boldsymbol{\Gamma}_p = \textbf{I}* 25$
  
        \item $\sigma_p = 2.5$

        \item $\phi_s = 1$
        \item $\psi_s = 2.5 $

        \item $\boldsymbol{\delta}_t = [5, 5, 5, 5, 10, 15, 0]^\top$
        \item $\boldsymbol{\Gamma}_t = \textbf{I}* 10$
        \item $\sigma_t = 2.5$

        \item $\alpha_q = 1$
        \item $\beta_q = 1$

\end{itemize}

\subsubsection{DQN}

\begin{itemize}
    \item Discount factor: .2
    \item Learning starts: 1,500
    \item Batch size: 32
    \item Learning rate: 5e-4
    \item Training iterations: 50,000
    \item Exploration fraction: 99\% annealed to 5\% over the first 35\% of training iterations

\end{itemize}
